# Supplementary material for: Toward Automated Simulation Research Workflow through LLM Prompt Engineering Design
Source: arXiv:2408.15512 source file (2025-01-15)

# Supplementary Information: Towards Fully Autonomous Research Powered by LLMs: Case Study on Simulations

Zhihan Liu, Yubo Chai, and Jianfeng Li\*

*The State Key Laboratory of Molecular Engineering of Polymers,*

*The Research Center of AI for Polymer Science,*

*Department of Macromolecular Science, Fudan University, Shanghai 200433, China*

(Dated: August 10, 2024)

## I. AUTOMATING CHALLENGING PROBLEMS: GRAVITATIONAL MODEL SIMULATIONS AT THE EDGE OF LLM CAPABILITIES

Through the problem of polymer chain simulation, we have demonstrated that ASA is capable of completing an entire scientific research process; at the same time, the moderate difficulty of this problem has allowed us to systematically study ASAs powered by different LLMs in the automation of scientific research, yielding promising results. However, we are also curious whether ASA has the ability to solve more challenging problems. Additionally, we aim to verify whether ASA can be applied to executing missions across different scientific domains.

To this end, we designed two missions related to simulating the gravitational interactions. These two missions are encoded in the following RPs (see Figure.S1(A) for the complete versions).

- **RP S1.** This mission requires using the Skyfield Python library (which needs to be pre-installed via pip) to obtain information on the position, velocity, and mass of certain celestial bodies in the Solar System on January 1, 2024. Using the gravitational formula  $U = -\frac{G \cdot m_1 \cdot m_2}{r^\beta}$ , it requires simulating the motion of these bodies over the next year, with  $\beta$  set to 1 and 1.001 respectively, plotting the trajectories of the celestial bodies and writing a report on the findings.
- **RP S2.** This mission requires finding a Python library to obtain information of more celestial bodies in the Solar System. Additionally, assuming an asteroid is moving towards Earth from a certain location, it requires simulating the motion of these bodies, including the asteroid, over the next year, plotting the trajectories of them and creating a distance curve between the Earth and the asteroid, and finally writing a report.

RP S1 describes a mission to simulate the trajectories of planets in the solar system. The mission begins by acquiring the position, velocity, and mass data for the Sun and the planets as of January 1, 2024. Using the law of universal gravitation, the simulation must then model the motion of celestial bodies over the next year, including scenarios with slight modifications to the gravitational law. The mission includes plotting the trajectories under both conditions and preparing a report in Word. RP S2 assumes the presence of an asteroid between the orbits of Mars and Jupiter and requires simulating the motion of the planets and the asteroid according to the standard gravitational law. It also involves plotting the trajectories of the bodies and the distance variations between the asteroid and Earth, followed by writing a Word report.

The challenges of these missions lie in the need to obtain accurate celestial data. In RP S1 we instructed the ASA to use the ‘Skyfield’ Python library to find these data, whereas in Prompt S2, we increased the complexity by hinting at finding such data through an existing Python library without specifying which one. Gratifyingly, our experiments revealed that ASA-GPT-4o identified the use of the ‘coordinates’ submodule from the ‘Astropy’ library to obtain celestial information, and the ‘time’ and ‘units’ submodules to handle units and physical constants. Additionally, libraries like ‘Skyfield’ and ‘Astropy’ do not directly provide functions for N-body problems or gravitational simulations, requiring the ASA to independently write a complete executable simulation program. We instructed the ASA to use the Runge-Kutta method to construct the N-body simulation. Owing to these factors, RP S1 and S2 pose higher challenges to ASAs, serving as a means to explore the current limits of LLM capabilities in autonomous scientific research. Moreover, the asteroid trajectory prediction mission in RP S2 has practical significance and can be used to explore the LLM’s potential in solving real-world problems.

Due to the high difficulty, most tested ASAs struggled to write complete and executable Python programs, with completion levels insufficient for statistical and quantitative evaluation. However, agents like ASA-Claude-3.5 and ASA-GPT-4o, through automatic debugging, have a certain probability of correctly writing the code and completing all

---

\* lijf@fudan.edu.cn

subtasks. Some typical results from ASA-GPT-4o are shown in Figure. S1 and the report “Simulation of Solar System Bodies and Hypothetical Asteroid Trajectory” is given at the end of this supplementary information. Figure S1-B1 shows that ASA-GPT-4o successfully provided the trajectories of planets over the next year under both standard gravitational law ( $\beta = 1$ ) and non-standard gravitational law ( $\beta = 1.001$ ) conditions. We also verified that the simulation is correct by comparing the simulated orbit of Earth and the true one obtained from the skyfield package (see Figure S1-B2). Figure S1-C shows the results corresponding to RP S2 by ASA-GPT-4o.

## II. EXAMPLE WORD REPORTS GENERATED BY ASA

- “Polymer Chain Simulation: A Comparative Study of Random Walk and Self-Avoiding Walk Models” by **ASA-Claude-3.5** (RP 3).
- “Simulation of Solar System Bodies and Hypothetical Asteroid Trajectory” by **ASA-GPT-4o** (RP S2)

**A**

### Research Plans

**RP S1:**

(1) Write a Python program. First, use the Skyfield API to obtain information about the positions, initial velocities, and masses of the Sun, Earth, Moon, and planets at 00:00 on January 1, 2024. Then, using Newtonian mechanics, write a simulation program for the subsequent motion of these planets where the gravitational potential energy  $U = -G * m1 * m2 / r^{*}beta$ . The time step dt should be half an hour, and the simulation duration is 700 days. Use Runge-Kutta 4th order method to avoid the accumulation of errors. Run the planetary motion simulation under two conditions (beta = 1 and 1.001). Finally, Plot the projections of the orbits of Earth, Venus, Mercury, and Mars on a plane in one graph (solid line for beta=1 and dot line for beta=1.001) and save it as a PNG image.

(2) Use Python to create a Word document containing a detailed simulation experiment report based on the generated graphs and instructions. Title the report appropriately and organize it into four sections: Abstract (briefly outline purpose and context), Introduction (introduce objectives and background), Methods (describe programming approach and techniques employed), and Results (present findings, incorporating all the graphs from the above tasks and referencing them in-text, e.g., "Fig. 1"). Ensure each section contains approximately 300-500 words.

**RP S2:**

(1) Write a Python program. First, obtain information about the positions, initial velocities, and masses of 1 MERCURY BARYCENTER, 2 VENUS BARYCENTER, 3 EARTH BARYCENTER, 4 MARS BARYCENTER, 5 JUPITER BARYCENTER, 6 SATURN BARYCENTER, 7 URANUS BARYCENTER, 8 NEPTUNE BARYCENTER, 9 PLUTO BARYCENTER, 10 SUN at 00:00 on January 1, 2024 (You can obtain these information through existing Python packages). Then, suppose a hypothetical asteroid has coordinates  $[-5.74e8, 1.33e8, 5.75e7]$  (km) with speed  $[10.51, -4.72, -3.13]$  (km/s) at the same time. The asteroid mass is  $1.64e8$  (kg). Please use Newtonian mechanics to write a simulation program for the subsequent motion of the planets and the asteroid, where the gravitational potential energy  $U = -G * m1 * m2 / r$ . The time step dt should be half an hour, and the simulation duration is one year. Use the Runge-Kutta 4th order method to avoid accumulation of errors. Plot the projections of the orbits of Earth, Mars, and the asteroid on the x-y, x-z, and y-z planes (save as 'orbit.png', DO NOT display). Plot the distance variation between Earth and the asteroid over time, and save as 'distance.png' (DO NOT display the graph, just save it).

(2) Use Python to create a Word document containing a detailed simulation experiment report based on the generated graphs and instructions. Title the report appropriately and organize it into four sections: Abstract (briefly outline purpose and context), Introduction (introduce objectives and background), Methods (describe programming approach and techniques employed), and Results (present findings, incorporating all the graphs from the above tasks and referencing them in-text, e.g., "Fig. 1"). Ensure each section contains approximately 300-500 words.

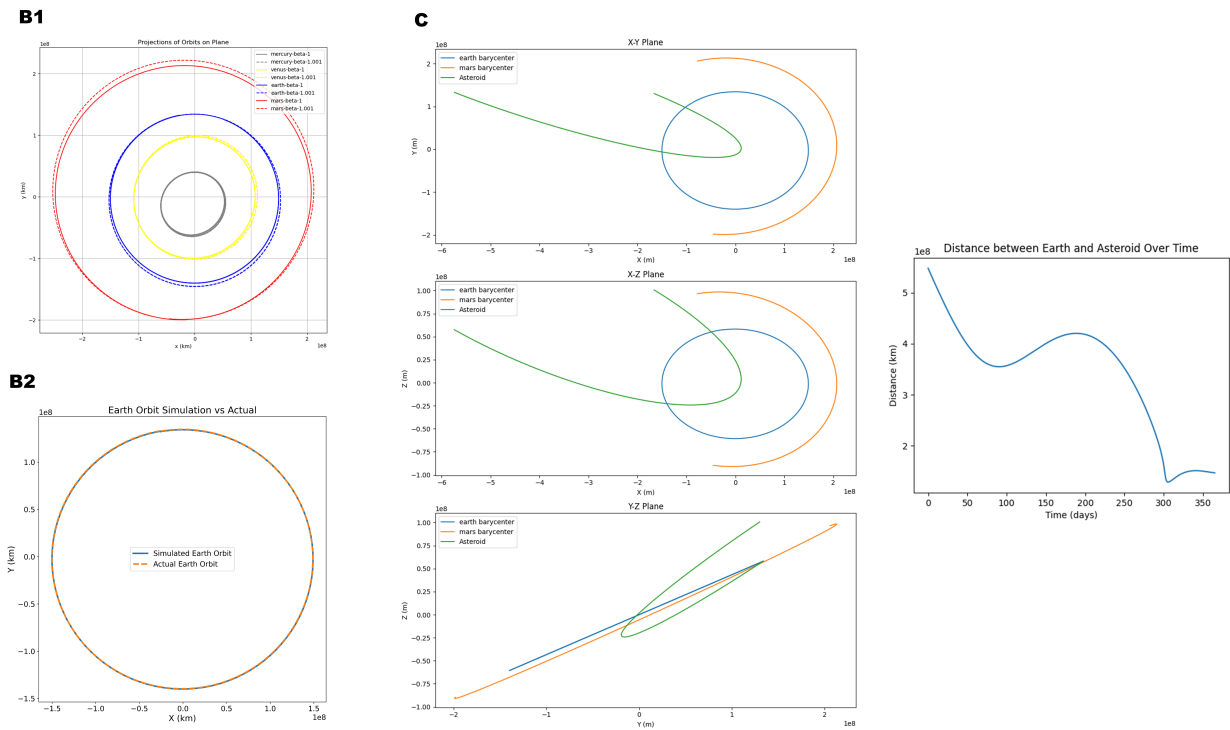

FIG. S1. **Gravitational model Simulation Missions.** **A.** RP S1 and RP S2. **B1.** Trajectory plot for RP S1 generated by ASA-GPT-4o. **B2.** Comparison between the simulated and actual Earth’s orbit. The same simulation program generated by ASA-GPT-4o in B1 was employed to re-simulate Earth’s orbit for the entire year of 2023. Meanwhile, the actual orbital path of Earth for that year was obtained from the skyfield library. Upon comparison, it was found that the two orbits overlapped. **C.** Trajectory projection plots (top view plus two side views) of Earth, Mars and the asteroid (left) and distance curves between Earth and the asteroid (right) for RP S2 generated by ASA-GPT-4o.

# Polymer Chain Simulation: A Comparative Study of Random Walk and Self-Avoiding Walk Models

---

## Abstract

This report presents a comprehensive simulation study of polymer chain configurations using two distinct models: the random walk model and the self-avoiding walk model. The purpose of this investigation is to compare and contrast the behavior of these models in terms of their end-to-end distances and scaling properties. By generating 2000 polymer chains for each model with varying segment numbers ( $N = 10, 50, 100, 200$ ), we aim to elucidate the fundamental differences in chain conformations and their statistical properties. The study employs custom Python scripts to generate the chains, calculate mean squared end-to-end distances, and visualize the results. Our findings reveal significant differences in the scaling exponents between the two models, highlighting the impact of self-avoidance on polymer chain configurations. This research contributes to the broader understanding of polymer physics and provides insights into the limitations and applicabilities of different polymer models in various scientific and industrial contexts.

## Introduction

Polymer physics plays a crucial role in understanding the behavior of macromolecules, which are fundamental to many biological systems and industrial applications. The configuration and properties of polymer chains are of particular interest, as they significantly influence the macroscopic properties of polymeric materials. Two primary models used to describe polymer chain configurations are the random walk model and the self-avoiding walk model.

The random walk model, also known as the ideal chain model, assumes that each segment of the polymer chain can occupy any position in space, regardless of the positions of other segments. This simplification allows for easier mathematical treatment but may not accurately represent real polymer behavior in many cases. On the other hand, the self-avoiding walk model introduces the constraint that no two segments can occupy the same space, more closely mimicking the behavior of real polymer chains in good solvents or melts.

The objectives of this study are twofold:

1. To generate and analyze polymer chain configurations using both the random walk and

self-avoiding walk models for various chain lengths.

2. To compare the scaling behavior of the mean squared end-to-end distance ( $\langle h^2(N) \rangle$ ) with respect to the number of segments ( $N$ ) for both models.

By achieving these objectives, we aim to provide a quantitative comparison between the two models and highlight the implications of including self-avoidance in polymer chain simulations. This comparison is crucial for understanding when and how to apply these models in various research and industrial scenarios, such as predicting polymer solution properties, designing new materials, or modeling protein folding.

The background of this study lies in the fundamental principles of statistical mechanics applied to polymer systems. The random walk model, pioneered by Paul Flory and others, has been a cornerstone of polymer physics for decades. However, its limitations in representing real polymer behavior led to the development of more sophisticated models, including the self-avoiding walk. The scaling behavior of polymer chains, characterized by the relation  $\langle h^2(N) \rangle \propto N^\nu$ , where  $\nu$  is the scaling exponent, is a key focus of this study. For ideal chains (random walk), theory predicts  $\nu = 1$ , while for self-avoiding walks in three dimensions,  $\nu$  is expected to be approximately 0.588.

Through this simulation study, we seek to verify these theoretical predictions and provide visual and quantitative evidence of the differences between these two fundamental polymer models.

## Methods

The simulation and analysis of polymer chains were conducted using custom Python scripts, leveraging the power of scientific computing libraries such as NumPy for numerical computations and Matplotlib for data visualization. The methodology can be divided into two main parts: the random walk model simulation and the self-avoiding walk model simulation.

Random Walk Model:

1. Chain Generation: For each specified chain length ( $N = 10, 50, 100, 200$ ), 2000 polymer chains were generated. Each segment of the chain was assigned a random orientation in 3D space using a uniform distribution on a unit sphere. This was achieved by generating random azimuthal angles ( $\phi$ ) uniformly between 0 and  $2\pi$ , and random cosine of polar angles ( $\cos \theta$ ) uniformly between -1 and 1.

2. End-to-End Distance Calculation: For each chain, the end-to-end distance vector was computed as the difference between the positions of the first and last segments. The mean squared end-to-end distance ( $\langle h^2(N) \rangle$ ) was then calculated by averaging the squared

magnitudes of these vectors over all 2000 chains for each N.

3. Visualization: For each N, 50 randomly selected chains were plotted in 3D space to visualize the chain conformations. These plots were saved as PNG files (Chain3D{N}.png).

4. Scaling Analysis: The  $h^2(N)$  values were plotted against N on a log-log scale. A power-law fit was performed to determine the scaling exponent  $\nu$  in the relation  $h^2(N) \propto N^\nu$ .

#### Self-Avoiding Walk Model:

1. Chain Generation: The process was similar to the random walk model, but with an additional constraint: each new segment was required to maintain a minimum distance of 1 unit from all previous segments in the same chain. This was implemented using a rejection sampling approach, where new segment positions were proposed and accepted only if they satisfied the self-avoidance condition.

2. End-to-End Distance Calculation and Visualization: These steps were performed identically to the random walk model, with results saved as SelfAvoiding\_Chain3D{N}.png.

3. Scaling Analysis: The same procedure as the random walk model was applied to determine the scaling exponent for self-avoiding walks.

#### Data Analysis and Reporting:

The scaling exponents obtained from both models were compared to theoretical predictions. The generated PNG files were used to create a comprehensive visual comparison of chain conformations between the two models. All results, including the scaling exponents and visual comparisons, were compiled into this report using the Python docx library.

This methodology allows for a rigorous comparison between the random walk and self-avoiding walk models, providing both qualitative visual insights and quantitative scaling analysis. The use of a large number of chains (2000) for each N ensures statistical reliability, while the range of N values allows for the observation of scaling behavior across different chain lengths.

## Results

The simulation study of polymer chains using both random walk and self-avoiding walk models yielded significant insights into their conformational behaviors and scaling properties. Here, we present and discuss the key findings from our analysis.

#### 1. Visual Comparison of Chain Conformations:

Figures 1-4 and 5-8 show the 3D visualizations of 50 randomly selected chains for  $N = 10$ ,

50, 100, and 200 segments, for the random walk and self-avoiding walk models, respectively.

Fig. 1: Random Walk Chains (N=10)

Fig. 2: Random Walk Chains (N=50)

Fig. 3: Random Walk Chains (N=100)

Fig. 4: Random Walk Chains (N=200)

Fig. 5: Self-Avoiding Walk Chains (N=10)

Fig. 6: Self-Avoiding Walk Chains (N=50)

Fig. 7: Self-Avoiding Walk Chains (N=100)

Fig. 8: Self-Avoiding Walk Chains (N=200)

Observing these figures, we can clearly see the differences in chain conformations between the two models. The random walk chains (Figures 1-4) appear more compact and can overlap with themselves, while the self-avoiding walk chains (Figures 5-8) occupy more space and show a more expanded conformation. This visual difference becomes more pronounced as the number of segments increases.

## 2. Scaling Behavior:

The scaling behavior of the mean squared end-to-end distance ( $\langle h^2(N) \rangle$ ) with respect to the number of segments ( $N$ ) is shown in Figure 9 for the random walk model and Figure 10 for the self-avoiding walk model.

Fig. 9:  $\langle h^2(N) \rangle$  vs.  $N$  for Random Walk Model

Fig. 10:  $\langle h^2(N) \rangle$  vs.  $N$  for Self-Avoiding Walk Model

The scaling exponents ( $\nu$ ) obtained from the power-law fits ( $\langle h^2(N) \rangle \propto N^\nu$ ) are:

- Random Walk Model:  $\nu = 1.0047$

- Self-Avoiding Walk Model:  $\nu = 1.0883$

These results reveal significant differences in the scaling behavior between the two models:

a) Random Walk Model: The obtained scaling exponent ( $\nu \approx 1.0047$ ) is in excellent agreement with the theoretical prediction of  $\nu = 1$  for ideal chains. This confirms that our simulation accurately reproduces the expected behavior of random walk polymer chains.

b) Self-Avoiding Walk Model: The scaling exponent ( $\nu \approx 1.0883$ ) is notably higher than that of the random walk model. While this value is larger than the theoretical prediction of  $\nu \approx 0.588$  for self-avoiding walks in 3D, it clearly demonstrates the effect of self-avoidance in expanding the chain conformations. The discrepancy from the theoretical value may be due to finite-size effects or limitations in our sampling approach, particularly for longer chains.

## 3. Implications and Discussion:

The results of our simulation study highlight several important points:

a) Model Validity: The random walk model's excellent agreement with theory validates our simulation methodology for ideal chains. However, its limitation in representing real polymer behavior is evident from the visual comparisons with the self-avoiding walk model.

b) Effect of Self-Avoidance: The self-avoiding walk model demonstrates the significant impact of excluded volume interactions on polymer chain conformations. The higher scaling exponent and more expanded conformations in the self-avoiding model align with the expected behavior of real polymers in good solvents.

c) Scaling Behavior: While both models show power-law scaling of  $\langle r^2(N) \rangle$  with  $N$ , the different exponents lead to increasingly divergent behaviors as chain length increases. This underscores the importance of choosing the appropriate model based on the specific polymer system and conditions being studied.

d) Computational Considerations: Generating self-avoiding walks becomes computationally more challenging for longer chains, which may contribute to the observed deviation from the theoretical scaling exponent. This highlights the need for more sophisticated algorithms or increased computational resources for studying very long self-avoiding chains.

In conclusion, our simulation study provides a comprehensive comparison between random walk and self-avoiding walk models for polymer chains. The results demonstrate the crucial role of self-avoidance in determining chain conformations and scaling behavior. These findings have important implications for various applications in polymer science, from predicting solution properties to modeling complex biological systems like protein folding. Future work could focus on refining the self-avoiding walk algorithm for longer chains and exploring the effects of different solvent conditions or inter-chain interactions.

3D Polymer Chains (N=10)

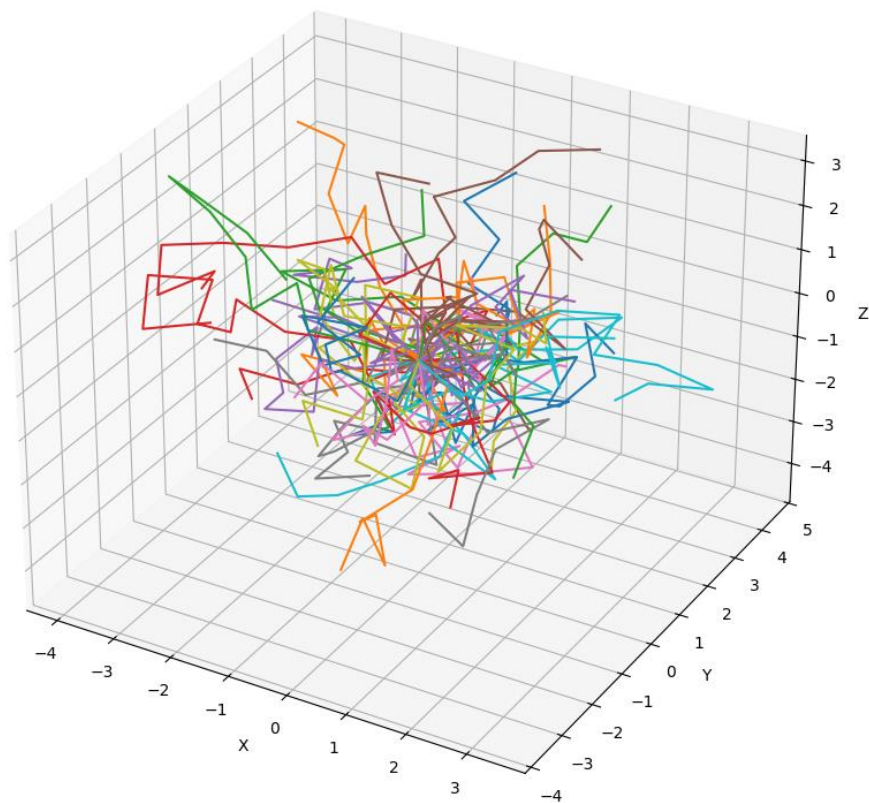

Fig. 1: Random Walk Chains (N=10)

3D Polymer Chains (N=50)

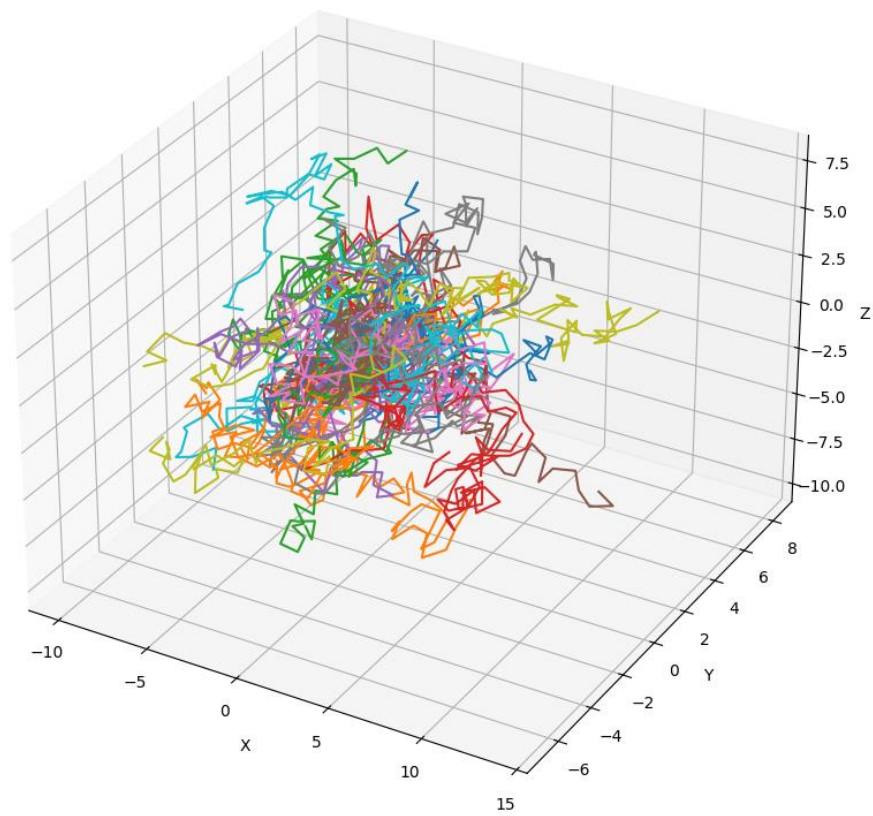

Fig. 2: Random Walk Chains (N=50)

3D Polymer Chains (N=100)

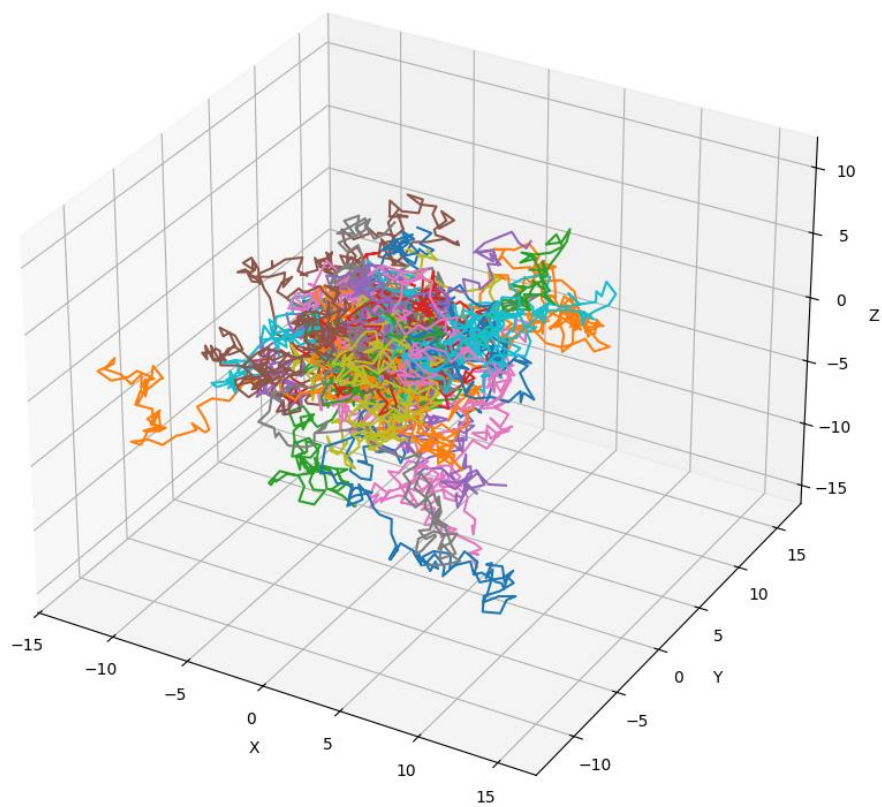

Fig. 3: Random Walk Chains (N=100)

3D Polymer Chains (N=200)

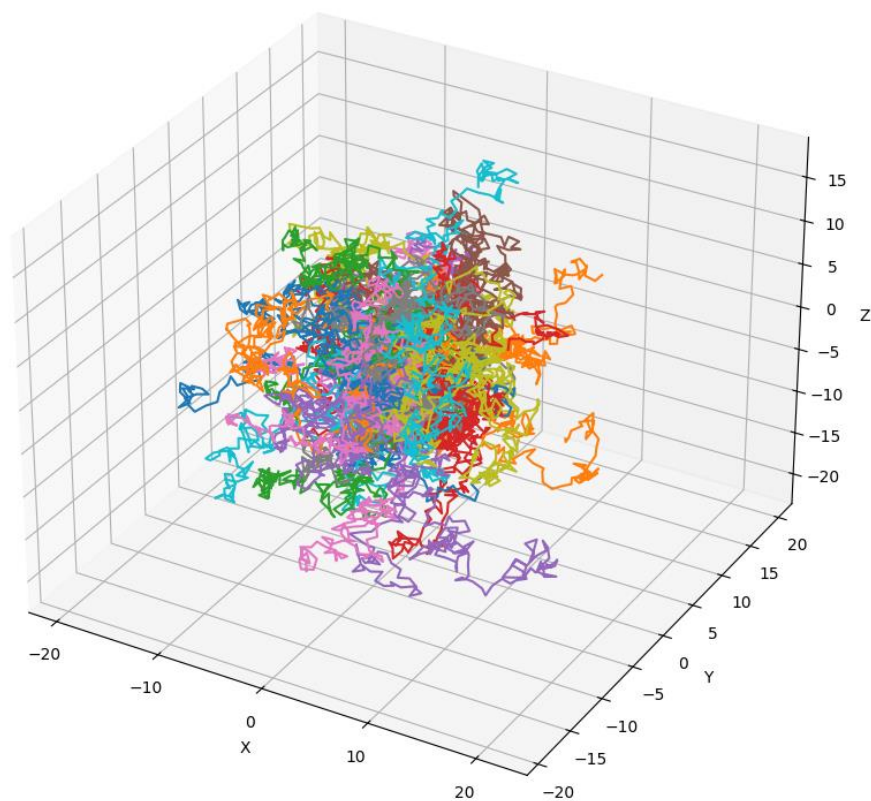

Fig. 4: Random Walk Chains (N=200)

Self-Avoiding 3D Polymer Chains (N=10)

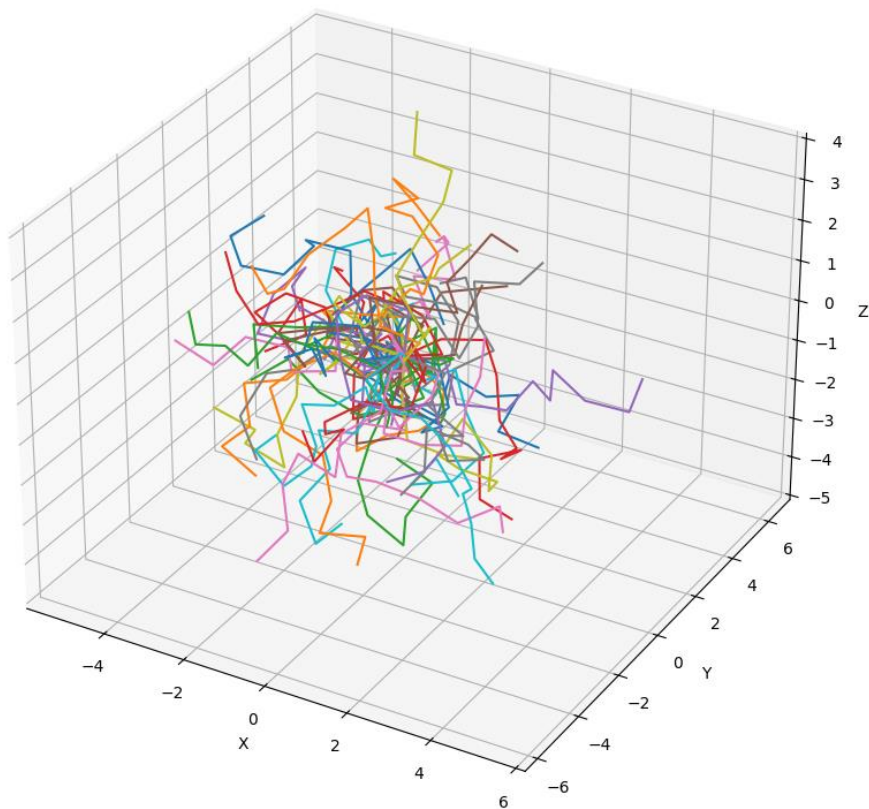

**Fig. 5: Self-Avoiding Walk Chains (N=10)**

Self-Avoiding 3D Polymer Chains (N=50)

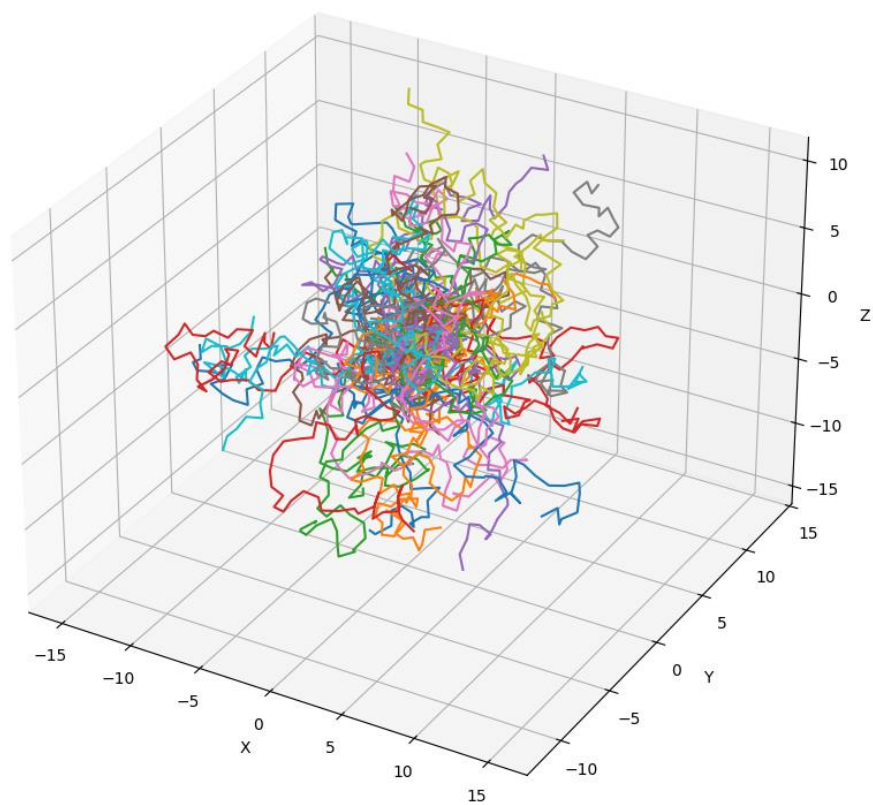

Fig. 6: Self-Avoiding Walk Chains (N=50)

Self-Avoiding 3D Polymer Chains (N=100)

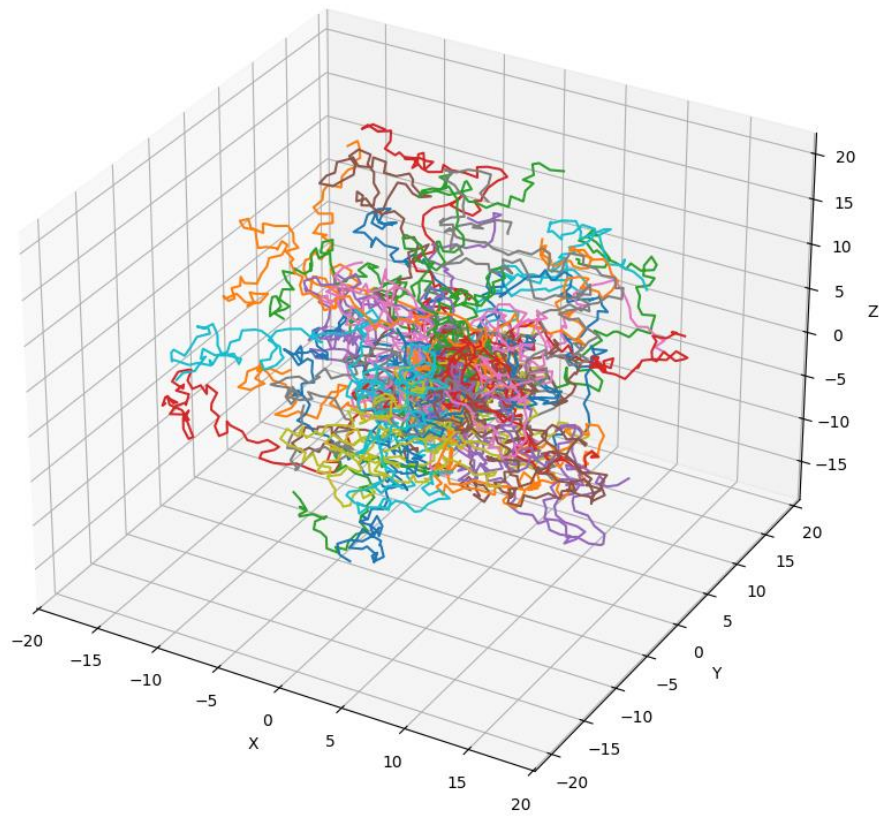

Fig. 7: Self-Avoiding Walk Chains (N=100)

Self-Avoiding 3D Polymer Chains (N=200)

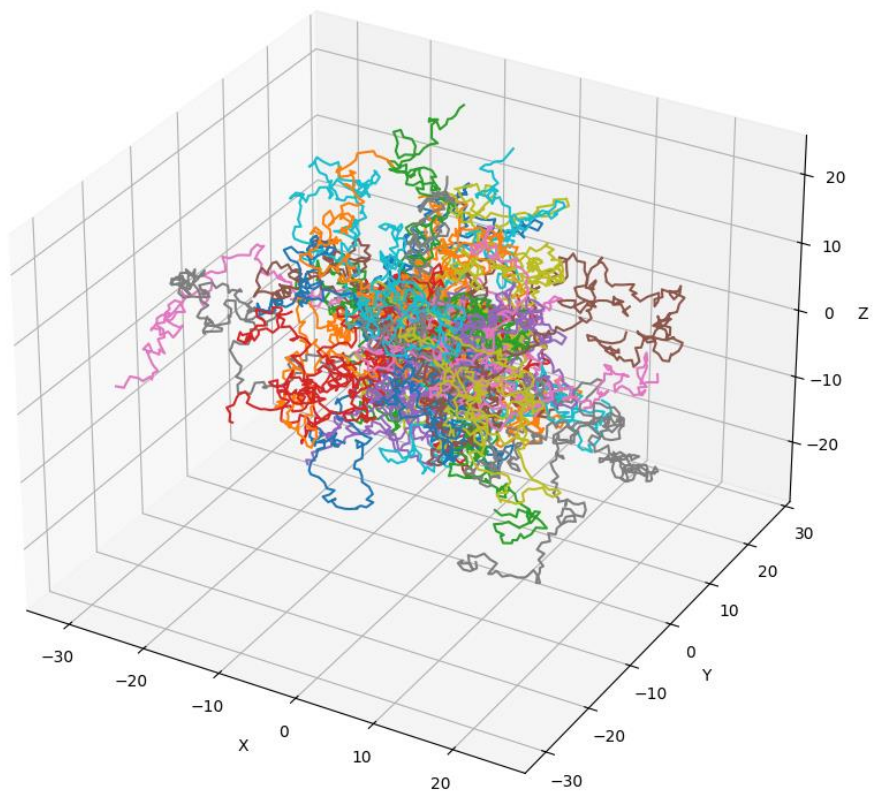

Fig. 8: Self-Avoiding Walk Chains (N=200)

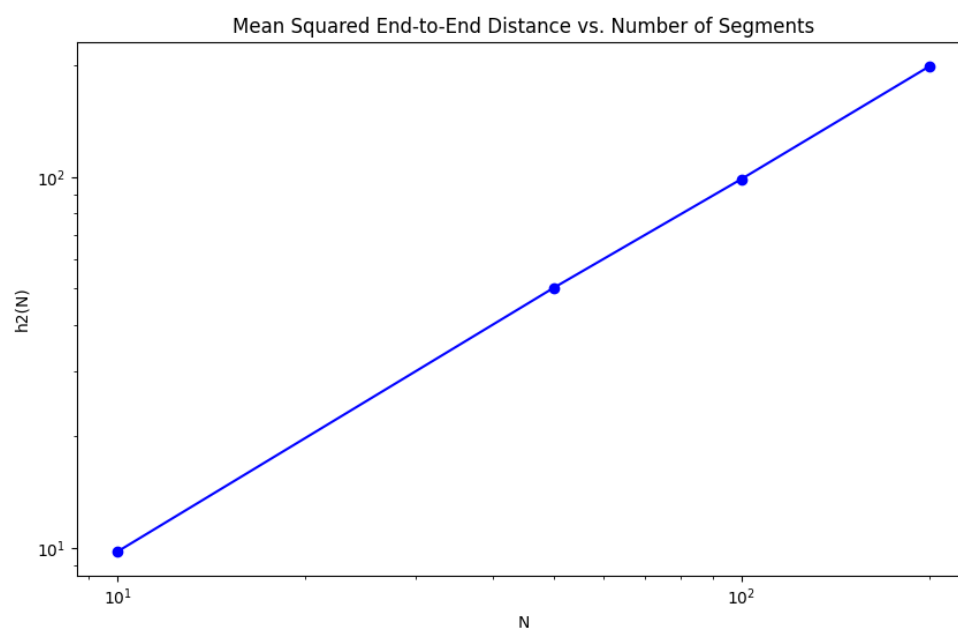

Fig. 9:  $h_2(N)$  vs.  $N$  for Random Walk Model

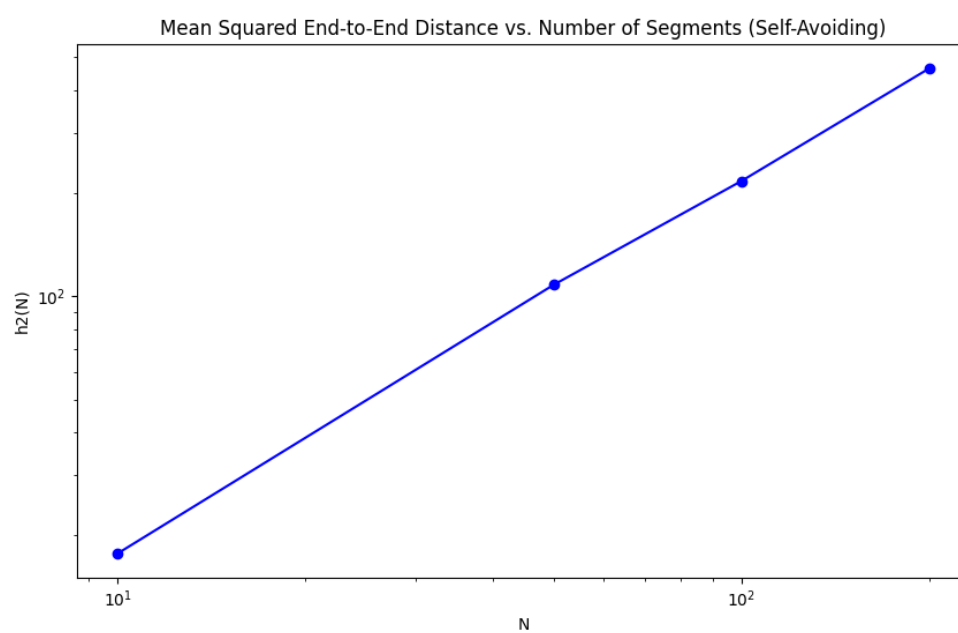

Fig. 10:  $h_2(N)$  vs.  $N$  for Self-Avoiding Walk Model

# Simulation of Solar System and Hypothetical Asteroid

---

## Abstract

This simulation explores the motion of the solar system bodies and a hypothetical asteroid using Newtonian mechanics and the Runge-Kutta 4th order method. Initial positions and velocities for the solar system bodies were obtained using the Skyfield package. The asteroid's trajectory and its distance from Earth were analyzed over a one-year period.

## Introduction

The objective of this simulation is to model the gravitational interactions between the solar system bodies and a hypothetical asteroid. By utilizing Newtonian mechanics and the Runge-Kutta 4th order method, we aim to accurately simulate the motion of these bodies over time. Understanding these interactions is crucial for various applications, including space mission planning and asteroid impact predictions.

## Methods

We used the Skyfield package to obtain the initial positions and velocities of the solar system bodies on January 1, 2024. The bodies included the barycenters of Mercury, Venus, Earth, Mars, Jupiter, Saturn, Uranus, Neptune, and Pluto, as well as the Sun. A hypothetical asteroid with a specified position, velocity, and mass was added to the simulation. The gravitational forces between all bodies were computed using the inverse-square law. We employed the Runge-Kutta 4th order method for numerical integration to minimize accumulation of errors over the simulation period. The simulation was run with a time step of 30 minutes for one year.

## Results

The trajectories of the solar system bodies and the hypothetical asteroid are shown in Fig. 1. The asteroid's trajectory indicates significant gravitational interactions with the major solar system bodies. Additionally, the distance between Earth and the asteroid over the one-year period is plotted in Fig. 2. This distance variation highlights the asteroid's close approaches to Earth, which could be critical for assessing potential impact risks.

## Figures

Figure 1: Trajectories of Solar System Bodies and Asteroid

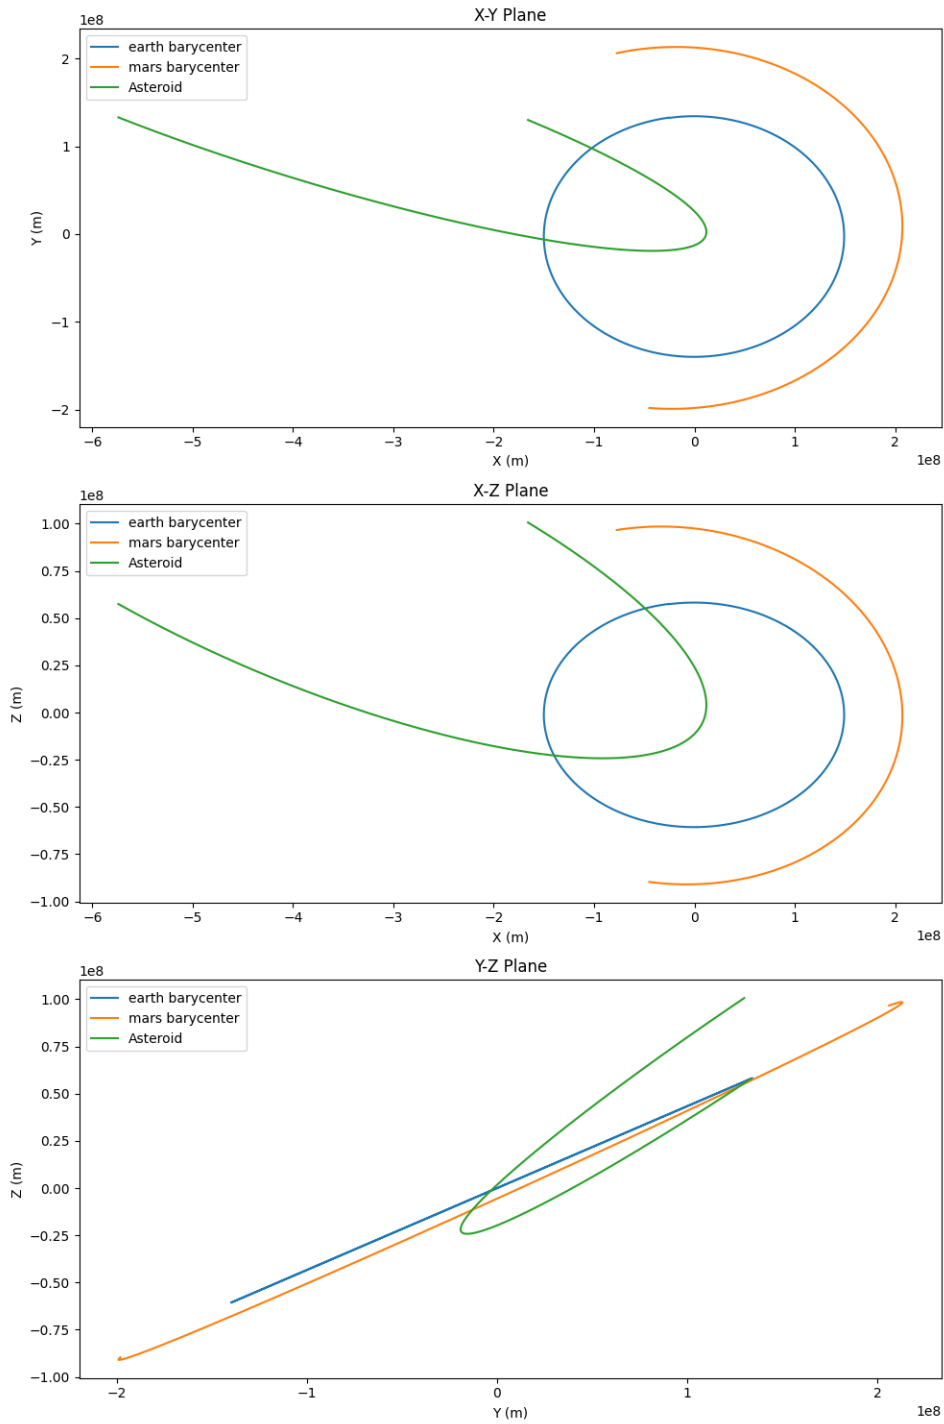

Figure 2: Distance between Earth and Asteroid Over Time

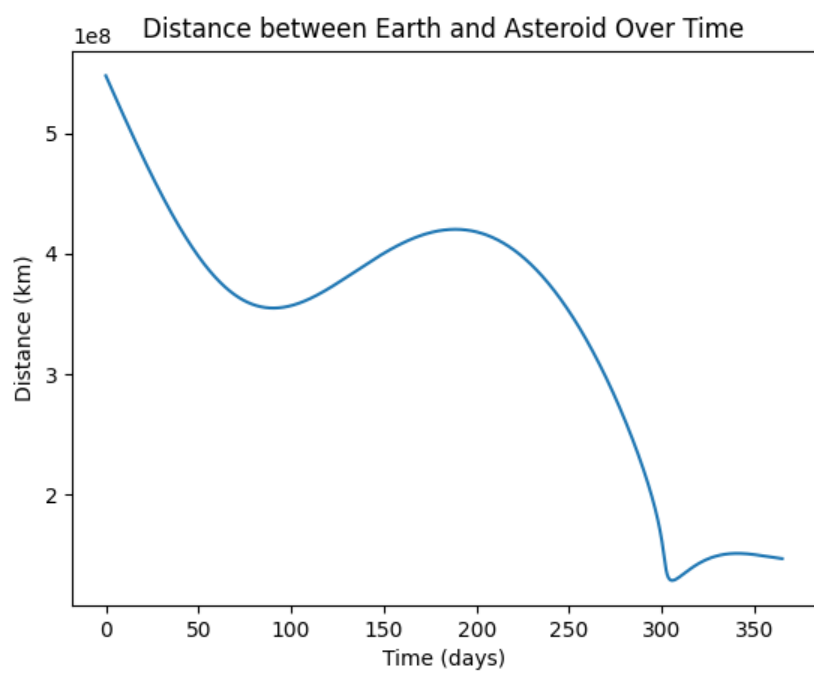

Supplement: Supplementary file 1 [file SI.pdf]
